# Supplementary material for: Game Theoretic Mixed Experts for Combinational Adversarial Machine Learning
Source: arXiv:2211.14669 source file (2023-04-29)
Supplement: Supplementary file 2 [file oldAppendix.tex]

\begin{table}[]
\begin{tabular}{|cccccccc|}
\hline
\multicolumn{8}{|c|}{Full $\text{GaME}_2$ Table (CIFAR-10, $F_s$)}                                           \\ \hline
\multicolumn{1}{|c|}{}          & B1+B5   & B1+RF   & B1+VF   & B1+ST   & B1+SB   & B1+BVT  & B5+RF   \\ \hline
\multicolumn{1}{|c|}{APGD(RF)}  & 87.00\% & 87.00\% & 87.00\% & 87.00\% & 87.00\% & 87.00\% & 85.00\% \\
\multicolumn{1}{|c|}{APGD(SB)}  & 92.00\% & 92.00\% & 92.00\% & 92.00\% & 92.00\% & 92.00\% & 89.00\% \\
\multicolumn{1}{|c|}{APGD(ST)}  & 89.00\% & 89.00\% & 89.00\% & 89.00\% & 89.00\% & 89.00\% & 89.00\% \\
\multicolumn{1}{|c|}{APGD(VF)}  & 51.00\% & 51.00\% & 51.00\% & 51.00\% & 51.00\% & 51.00\% & 52.00\% \\
\multicolumn{1}{|c|}{MIME(B1)}  & 6.00\%  & 6.00\%  & 6.00\%  & 6.00\%  & 6.00\%  & 6.00\%  & 41.00\% \\
\multicolumn{1}{|c|}{MIME(B5)}  & 9.00\%  & 9.00\%  & 9.00\%  & 9.00\%  & 9.00\%  & 9.00\%  & 19.00\% \\
\multicolumn{1}{|c|}{MIME(BVT)} & 56.00\% & 56.00\% & 56.00\% & 56.00\% & 56.00\% & 56.00\% & 69.00\% \\
\multicolumn{1}{|c|}{S(B1,B5)}  & 5.00\%  & 5.00\%  & 5.00\%  & 5.00\%  & 5.00\%  & 5.00\%  & 41.00\% \\
\multicolumn{1}{|c|}{S(B1,BVT)} & 9.00\%  & 9.00\%  & 9.00\%  & 9.00\%  & 9.00\%  & 9.00\%  & 66.00\% \\
\multicolumn{1}{|c|}{S(B1,RF)}  & 9.00\%  & 9.00\%  & 9.00\%  & 9.00\%  & 9.00\%  & 9.00\%  & 60.00\% \\
\multicolumn{1}{|c|}{S(B1,SB)}  & 6.00\%  & 6.00\%  & 6.00\%  & 6.00\%  & 6.00\%  & 6.00\%  & 55.00\% \\
\multicolumn{1}{|c|}{S(B1,ST)}  & 19.00\% & 19.00\% & 19.00\% & 19.00\% & 19.00\% & 19.00\% & 73.00\% \\
\multicolumn{1}{|c|}{S(B1,VF)}  & 5.00\%  & 5.00\%  & 5.00\%  & 5.00\%  & 5.00\%  & 5.00\%  & 46.00\% \\
\multicolumn{1}{|c|}{S(B5,BVT)} & 22.00\% & 22.00\% & 22.00\% & 22.00\% & 22.00\% & 22.00\% & 35.00\% \\
\multicolumn{1}{|c|}{S(B5,RF)}  & 22.00\% & 22.00\% & 22.00\% & 22.00\% & 22.00\% & 22.00\% & 33.00\% \\
\multicolumn{1}{|c|}{S(B5,SB)}  & 25.00\% & 25.00\% & 25.00\% & 25.00\% & 25.00\% & 25.00\% & 31.00\% \\
\multicolumn{1}{|c|}{S(B5,ST)}  & 60.00\% & 60.00\% & 60.00\% & 60.00\% & 60.00\% & 60.00\% & 53.00\% \\
\multicolumn{1}{|c|}{S(B5,VF)}  & 10.00\% & 10.00\% & 10.00\% & 10.00\% & 10.00\% & 10.00\% & 19.00\% \\
\multicolumn{1}{|c|}{S(RF,BVT)} & 69.00\% & 69.00\% & 69.00\% & 69.00\% & 69.00\% & 69.00\% & 72.00\% \\
\multicolumn{1}{|c|}{S(RF,SB)}  & 90.00\% & 90.00\% & 90.00\% & 90.00\% & 90.00\% & 90.00\% & 87.00\% \\
\multicolumn{1}{|c|}{S(RF,ST)}  & 87.00\% & 87.00\% & 87.00\% & 87.00\% & 87.00\% & 87.00\% & 88.00\% \\
\multicolumn{1}{|c|}{S(RF,VF)}  & 58.00\% & 58.00\% & 58.00\% & 58.00\% & 58.00\% & 58.00\% & 58.00\% \\
\multicolumn{1}{|c|}{S(SB,BVT)} & 77.00\% & 77.00\% & 77.00\% & 77.00\% & 77.00\% & 77.00\% & 81.00\% \\
\multicolumn{1}{|c|}{S(SB,ST)}  & 91.00\% & 91.00\% & 91.00\% & 91.00\% & 91.00\% & 91.00\% & 89.00\% \\
\multicolumn{1}{|c|}{S(ST,BVT)} & 90.00\% & 90.00\% & 90.00\% & 90.00\% & 90.00\% & 90.00\% & 93.00\% \\
\multicolumn{1}{|c|}{S(VF,BVT)} & 50.00\% & 50.00\% & 50.00\% & 50.00\% & 50.00\% & 50.00\% & 62.00\% \\
\multicolumn{1}{|c|}{S(VF,SB)}  & 78.00\% & 78.00\% & 78.00\% & 78.00\% & 78.00\% & 78.00\% & 80.00\% \\
\multicolumn{1}{|c|}{S(VF,ST)}  & 83.00\% & 83.00\% & 83.00\% & 83.00\% & 83.00\% & 83.00\% & 92.00\% \\ \hline
\end{tabular}
\end{table}

\begin{table}[]
\begin{tabular}{|cccccccc|}
\hline
\multicolumn{8}{|c|}{Full $\text{GaME}_2$ Table (CIFAR-10, $F_s$)}                                           \\ \hline
\multicolumn{1}{|c|}{}          & B5+VF   & B5+ST   & B5+SB   & B5+BVT  & RF+VF   & RF+ST   & RF+SB   \\ \hline
\multicolumn{1}{|c|}{APGD(RF)}  & 85.00\% & 85.00\% & 85.00\% & 85.00\% & 46.00\% & 46.00\% & 46.00\% \\
\multicolumn{1}{|c|}{APGD(SB)}  & 89.00\% & 89.00\% & 89.00\% & 89.00\% & 79.00\% & 79.00\% & 79.00\% \\
\multicolumn{1}{|c|}{APGD(ST)}  & 89.00\% & 89.00\% & 89.00\% & 89.00\% & 83.00\% & 83.00\% & 83.00\% \\
\multicolumn{1}{|c|}{APGD(VF)}  & 52.00\% & 52.00\% & 52.00\% & 52.00\% & 75.00\% & 75.00\% & 75.00\% \\
\multicolumn{1}{|c|}{MIME(B1)}  & 41.00\% & 41.00\% & 41.00\% & 41.00\% & 82.00\% & 82.00\% & 82.00\% \\
\multicolumn{1}{|c|}{MIME(B5)}  & 19.00\% & 19.00\% & 19.00\% & 19.00\% & 82.00\% & 82.00\% & 82.00\% \\
\multicolumn{1}{|c|}{MIME(BVT)} & 69.00\% & 69.00\% & 69.00\% & 69.00\% & 83.00\% & 83.00\% & 83.00\% \\
\multicolumn{1}{|c|}{S(B1,B5)}  & 41.00\% & 41.00\% & 41.00\% & 41.00\% & 83.00\% & 83.00\% & 83.00\% \\
\multicolumn{1}{|c|}{S(B1,BVT)} & 66.00\% & 66.00\% & 66.00\% & 66.00\% & 84.00\% & 84.00\% & 84.00\% \\
\multicolumn{1}{|c|}{S(B1,RF)}  & 60.00\% & 60.00\% & 60.00\% & 60.00\% & 54.00\% & 54.00\% & 54.00\% \\
\multicolumn{1}{|c|}{S(B1,SB)}  & 55.00\% & 55.00\% & 55.00\% & 55.00\% & 80.00\% & 80.00\% & 80.00\% \\
\multicolumn{1}{|c|}{S(B1,ST)}  & 73.00\% & 73.00\% & 73.00\% & 73.00\% & 81.00\% & 81.00\% & 81.00\% \\
\multicolumn{1}{|c|}{S(B1,VF)}  & 46.00\% & 46.00\% & 46.00\% & 46.00\% & 79.00\% & 79.00\% & 79.00\% \\
\multicolumn{1}{|c|}{S(B5,BVT)} & 35.00\% & 35.00\% & 35.00\% & 35.00\% & 83.00\% & 83.00\% & 83.00\% \\
\multicolumn{1}{|c|}{S(B5,RF)}  & 33.00\% & 33.00\% & 33.00\% & 33.00\% & 56.00\% & 56.00\% & 56.00\% \\
\multicolumn{1}{|c|}{S(B5,SB)}  & 31.00\% & 31.00\% & 31.00\% & 31.00\% & 80.00\% & 80.00\% & 80.00\% \\
\multicolumn{1}{|c|}{S(B5,ST)}  & 53.00\% & 53.00\% & 53.00\% & 53.00\% & 82.00\% & 82.00\% & 82.00\% \\
\multicolumn{1}{|c|}{S(B5,VF)}  & 19.00\% & 19.00\% & 19.00\% & 19.00\% & 78.00\% & 78.00\% & 78.00\% \\
\multicolumn{1}{|c|}{S(RF,BVT)} & 72.00\% & 72.00\% & 72.00\% & 72.00\% & 56.00\% & 56.00\% & 56.00\% \\
\multicolumn{1}{|c|}{S(RF,SB)}  & 87.00\% & 87.00\% & 87.00\% & 87.00\% & 50.00\% & 50.00\% & 50.00\% \\
\multicolumn{1}{|c|}{S(RF,ST)}  & 88.00\% & 88.00\% & 88.00\% & 88.00\% & 70.00\% & 70.00\% & 70.00\% \\
\multicolumn{1}{|c|}{S(RF,VF)}  & 58.00\% & 58.00\% & 58.00\% & 58.00\% & 50.00\% & 50.00\% & 50.00\% \\
\multicolumn{1}{|c|}{S(SB,BVT)} & 81.00\% & 81.00\% & 81.00\% & 81.00\% & 80.00\% & 80.00\% & 80.00\% \\
\multicolumn{1}{|c|}{S(SB,ST)}  & 89.00\% & 89.00\% & 89.00\% & 89.00\% & 82.00\% & 82.00\% & 82.00\% \\
\multicolumn{1}{|c|}{S(ST,BVT)} & 93.00\% & 93.00\% & 93.00\% & 93.00\% & 85.00\% & 85.00\% & 85.00\% \\
\multicolumn{1}{|c|}{S(VF,BVT)} & 62.00\% & 62.00\% & 62.00\% & 62.00\% & 77.00\% & 77.00\% & 77.00\% \\
\multicolumn{1}{|c|}{S(VF,SB)}  & 80.00\% & 80.00\% & 80.00\% & 80.00\% & 77.00\% & 77.00\% & 77.00\% \\
\multicolumn{1}{|c|}{S(VF,ST)}  & 92.00\% & 92.00\% & 92.00\% & 92.00\% & 82.00\% & 82.00\% & 82.00\% \\ \hline
\end{tabular}
\end{table}

\begin{table}[]
\begin{tabular}{|cccccccc|}
\hline
\multicolumn{8}{|c|}{Full $\text{GaME}_2$ Table (CIFAR-10, $F_s$)}                                           \\ \hline
\multicolumn{1}{|c|}{}          & RF+BVT  & VF+ST   & VF+SB   & VF+BVT  & ST+SB   & ST+BVT  & SB+BVT  \\ \hline
\multicolumn{1}{|c|}{APGD(RF)}  & 46.00\% & 79.00\% & 79.00\% & 79.00\% & 60.00\% & 60.00\% & 57.00\% \\
\multicolumn{1}{|c|}{APGD(SB)}  & 79.00\% & 88.00\% & 88.00\% & 88.00\% & 55.00\% & 55.00\% & 1.00\%  \\
\multicolumn{1}{|c|}{APGD(ST)}  & 83.00\% & 94.00\% & 94.00\% & 94.00\% & 0.00\%  & 0.00\%  & 78.00\% \\
\multicolumn{1}{|c|}{APGD(VF)}  & 75.00\% & 26.00\% & 26.00\% & 26.00\% & 54.00\% & 54.00\% & 56.00\% \\
\multicolumn{1}{|c|}{MIME(B1)}  & 82.00\% & 94.00\% & 94.00\% & 94.00\% & 70.00\% & 70.00\% & 81.00\% \\
\multicolumn{1}{|c|}{MIME(B5)}  & 82.00\% & 93.00\% & 93.00\% & 93.00\% & 61.00\% & 61.00\% & 80.00\% \\
\multicolumn{1}{|c|}{MIME(BVT)} & 83.00\% & 91.00\% & 91.00\% & 91.00\% & 68.00\% & 68.00\% & 82.00\% \\
\multicolumn{1}{|c|}{S(B1,B5)}  & 83.00\% & 94.00\% & 94.00\% & 94.00\% & 74.00\% & 74.00\% & 80.00\% \\
\multicolumn{1}{|c|}{S(B1,BVT)} & 84.00\% & 94.00\% & 94.00\% & 94.00\% & 66.00\% & 66.00\% & 75.00\% \\
\multicolumn{1}{|c|}{S(B1,RF)}  & 54.00\% & 87.00\% & 87.00\% & 87.00\% & 63.00\% & 63.00\% & 75.00\% \\
\multicolumn{1}{|c|}{S(B1,SB)}  & 80.00\% & 89.00\% & 89.00\% & 89.00\% & 56.00\% & 56.00\% & 6.00\%  \\
\multicolumn{1}{|c|}{S(B1,ST)}  & 81.00\% & 93.00\% & 93.00\% & 93.00\% & 0.00\%  & 0.00\%  & 83.00\% \\
\multicolumn{1}{|c|}{S(B1,VF)}  & 79.00\% & 72.00\% & 72.00\% & 72.00\% & 66.00\% & 66.00\% & 72.00\% \\
\multicolumn{1}{|c|}{S(B5,BVT)} & 83.00\% & 94.00\% & 94.00\% & 94.00\% & 64.00\% & 64.00\% & 81.00\% \\
\multicolumn{1}{|c|}{S(B5,RF)}  & 56.00\% & 86.00\% & 86.00\% & 86.00\% & 62.00\% & 62.00\% & 72.00\% \\
\multicolumn{1}{|c|}{S(B5,SB)}  & 80.00\% & 90.00\% & 90.00\% & 90.00\% & 57.00\% & 57.00\% & 9.00\%  \\
\multicolumn{1}{|c|}{S(B5,ST)}  & 82.00\% & 93.00\% & 93.00\% & 93.00\% & 0.00\%  & 0.00\%  & 82.00\% \\
\multicolumn{1}{|c|}{S(B5,VF)}  & 78.00\% & 68.00\% & 68.00\% & 68.00\% & 69.00\% & 69.00\% & 75.00\% \\
\multicolumn{1}{|c|}{S(RF,BVT)} & 56.00\% & 82.00\% & 82.00\% & 82.00\% & 61.00\% & 61.00\% & 67.00\% \\
\multicolumn{1}{|c|}{S(RF,SB)}  & 50.00\% & 80.00\% & 80.00\% & 80.00\% & 50.00\% & 50.00\% & 1.00\%  \\
\multicolumn{1}{|c|}{S(RF,ST)}  & 70.00\% & 92.00\% & 92.00\% & 92.00\% & 0.00\%  & 0.00\%  & 73.00\% \\
\multicolumn{1}{|c|}{S(RF,VF)}  & 50.00\% & 34.00\% & 34.00\% & 34.00\% & 53.00\% & 53.00\% & 52.00\% \\
\multicolumn{1}{|c|}{S(SB,BVT)} & 80.00\% & 89.00\% & 89.00\% & 89.00\% & 52.00\% & 52.00\% & 3.00\%  \\
\multicolumn{1}{|c|}{S(SB,ST)}  & 82.00\% & 92.00\% & 92.00\% & 92.00\% & 0.00\%  & 0.00\%  & 36.00\% \\
\multicolumn{1}{|c|}{S(ST,BVT)} & 85.00\% & 94.00\% & 94.00\% & 94.00\% & 0.00\%  & 0.00\%  & 80.00\% \\
\multicolumn{1}{|c|}{S(VF,BVT)} & 77.00\% & 53.00\% & 53.00\% & 53.00\% & 61.00\% & 61.00\% & 68.00\% \\
\multicolumn{1}{|c|}{S(VF,SB)}  & 77.00\% & 78.00\% & 78.00\% & 78.00\% & 48.00\% & 48.00\% & 0.00\%  \\
\multicolumn{1}{|c|}{S(VF,ST)}  & 82.00\% & 82.00\% & 82.00\% & 82.00\% & 1.00\%  & 1.00\%  & 78.00\% \\ \hline
\end{tabular}
\end{table}

\begin{table}[]
\begin{tabular}{|cccccccc|}
\hline
\multicolumn{8}{|c|}{Full $\text{GaME}_2$ Table (CIFAR-10, $F_h$)}                                                                            \\ \hline
\multicolumn{1}{|c|}{Attack}    & B1+B5   & B1+RF   & B1+VF   & B1+ST   & B1+SB   & B1+BVT  & B5+RF   \\
\multicolumn{1}{|c|}{APGD(RF)}  & 87.00\% & 71.00\% & 78.00\% & 69.00\% & 71.00\% & 80.00\% & 61.00\% \\
\multicolumn{1}{|c|}{APGD(SB)}  & 89.00\% & 84.00\% & 92.00\% & 67.00\% & 44.00\% & 86.00\% & 82.00\% \\
\multicolumn{1}{|c|}{APGD(ST)}  & 90.00\% & 86.00\% & 93.00\% & 42.00\% & 84.00\% & 89.00\% & 86.00\% \\
\multicolumn{1}{|c|}{APGD(VF)}  & 52.00\% & 65.00\% & 34.00\% & 57.00\% & 50.00\% & 40.00\% & 63.00\% \\
\multicolumn{1}{|c|}{MIME(B1)}  & 24.00\% & 42.00\% & 60.00\% & 37.00\% & 45.00\% & 51.00\% & 62.00\% \\
\multicolumn{1}{|c|}{MIME(B5)}  & 14.00\% & 41.00\% & 52.00\% & 33.00\% & 47.00\% & 46.00\% & 45.00\% \\
\multicolumn{1}{|c|}{MIME(BVT)} & 63.00\% & 70.00\% & 69.00\% & 64.00\% & 66.00\% & 32.00\% & 78.00\% \\
\multicolumn{1}{|c|}{S(B1,B5)}  & 21.00\% & 46.00\% & 46.00\% & 36.00\% & 39.00\% & 53.00\% & 62.00\% \\
\multicolumn{1}{|c|}{S(B1,BVT)} & 46.00\% & 37.00\% & 55.00\% & 31.00\% & 41.00\% & 17.00\% & 74.00\% \\
\multicolumn{1}{|c|}{S(B1,RF)}  & 33.00\% & 29.00\% & 45.00\% & 39.00\% & 43.00\% & 52.00\% & 59.00\% \\
\multicolumn{1}{|c|}{S(B1,SB)}  & 26.00\% & 42.00\% & 46.00\% & 30.00\% & 7.00\%  & 49.00\% & 67.00\% \\
\multicolumn{1}{|c|}{S(B1,ST)}  & 44.00\% & 42.00\% & 56.00\% & 9.00\%  & 45.00\% & 48.00\% & 78.00\% \\
\multicolumn{1}{|c|}{S(B1,VF)}  & 28.00\% & 39.00\% & 37.00\% & 38.00\% & 43.00\% & 35.00\% & 60.00\% \\
\multicolumn{1}{|c|}{S(B5,BVT)} & 35.00\% & 48.00\% & 61.00\% & 42.00\% & 55.00\% & 22.00\% & 64.00\% \\
\multicolumn{1}{|c|}{S(B5,RF)}  & 27.00\% & 36.00\% & 65.00\% & 40.00\% & 46.00\% & 54.00\% & 42.00\% \\
\multicolumn{1}{|c|}{S(B5,SB)}  & 24.00\% & 54.00\% & 53.00\% & 37.00\% & 17.00\% & 50.00\% & 50.00\% \\
\multicolumn{1}{|c|}{S(B5,ST)}  & 54.00\% & 66.00\% & 76.00\% & 30.00\% & 66.00\% & 78.00\% & 69.00\% \\
\multicolumn{1}{|c|}{S(B5,VF)}  & 18.00\% & 49.00\% & 40.00\% & 36.00\% & 45.00\% & 35.00\% & 52.00\% \\
\multicolumn{1}{|c|}{S(RF,BVT)} & 72.00\% & 65.00\% & 77.00\% & 69.00\% & 66.00\% & 48.00\% & 62.00\% \\
\multicolumn{1}{|c|}{S(RF,SB)}  & 88.00\% & 72.00\% & 86.00\% & 66.00\% & 49.00\% & 77.00\% & 66.00\% \\
\multicolumn{1}{|c|}{S(RF,ST)}  & 87.00\% & 81.00\% & 90.00\% & 51.00\% & 78.00\% & 85.00\% & 76.00\% \\
\multicolumn{1}{|c|}{S(RF,VF)}  & 56.00\% & 58.00\% & 49.00\% & 58.00\% & 55.00\% & 47.00\% & 52.00\% \\
\multicolumn{1}{|c|}{S(SB,BVT)} & 78.00\% & 85.00\% & 79.00\% & 64.00\% & 33.00\% & 50.00\% & 81.00\% \\
\multicolumn{1}{|c|}{S(SB,ST)}  & 89.00\% & 85.00\% & 90.00\% & 42.00\% & 66.00\% & 90.00\% & 84.00\% \\
\multicolumn{1}{|c|}{S(ST,BVT)} & 91.00\% & 88.00\% & 90.00\% & 38.00\% & 84.00\% & 54.00\% & 90.00\% \\
\multicolumn{1}{|c|}{S(VF,BVT)} & 60.00\% & 67.00\% & 51.00\% & 59.00\% & 58.00\% & 27.00\% & 69.00\% \\
\multicolumn{1}{|c|}{S(VF,SB)}  & 78.00\% & 81.00\% & 80.00\% & 64.00\% & 41.00\% & 74.00\% & 77.00\% \\
\multicolumn{1}{|c|}{S(VF,ST)}  & 88.00\% & 82.00\% & 82.00\% & 40.00\% & 75.00\% & 77.00\% & 86.00\% \\ \hline
\end{tabular}
\end{table}

\begin{table}[]
\begin{tabular}{|crrrrrrr|}
\hline
\multicolumn{8}{|c|}{Full $\text{GaME}_2$ Table (CIFAR-10, $F_h$)}                                                                                                                                                                                                            \\ \hline
\multicolumn{1}{|c|}{Attack}    & \multicolumn{1}{l}{B5+VF} & \multicolumn{1}{l}{B5+ST} & \multicolumn{1}{l}{B5+SB} & \multicolumn{1}{l}{B5+BVT} & \multicolumn{1}{l}{RF+VF} & \multicolumn{1}{l}{RF+ST} & \multicolumn{1}{l|}{RF+SB} \\
\multicolumn{1}{|c|}{APGD(RF)}  & 81.00\%                   & 72.00\%                   & 74.00\%                   & 74.00\%                    & 63.00\%                   & 56.00\%                   & 48.00\%                    \\
\multicolumn{1}{|c|}{APGD(SB)}  & 88.00\%                   & 67.00\%                   & 46.00\%                   & 84.00\%                    & 84.00\%                   & 69.00\%                   & 40.00\%                    \\
\multicolumn{1}{|c|}{APGD(ST)}  & 91.00\%                   & 41.00\%                   & 84.00\%                   & 91.00\%                    & 88.00\%                   & 40.00\%                   & 83.00\%                    \\
\multicolumn{1}{|c|}{APGD(VF)}  & 41.00\%                   & 56.00\%                   & 60.00\%                   & 35.00\%                    & 49.00\%                   & 67.00\%                   & 65.00\%                    \\
\multicolumn{1}{|c|}{MIME(B1)}  & 72.00\%                   & 54.00\%                   & 62.00\%                   & 62.00\%                    & 86.00\%                   & 75.00\%                   & 82.00\%                    \\
\multicolumn{1}{|c|}{MIME(B5)}  & 58.00\%                   & 43.00\%                   & 46.00\%                   & 49.00\%                    & 86.00\%                   & 72.00\%                   & 83.00\%                    \\
\multicolumn{1}{|c|}{MIME(BVT)} & 81.00\%                   & 64.00\%                   & 80.00\%                   & 35.00\%                    & 88.00\%                   & 71.00\%                   & 88.00\%                    \\
\multicolumn{1}{|c|}{S(B1,B5)}  & 57.00\%                   & 63.00\%                   & 63.00\%                   & 64.00\%                    & 87.00\%                   & 80.00\%                   & 83.00\%                    \\
\multicolumn{1}{|c|}{S(B1,BVT)} & 81.00\%                   & 59.00\%                   & 75.00\%                   & 44.00\%                    & 89.00\%                   & 70.00\%                   & 83.00\%                    \\
\multicolumn{1}{|c|}{S(B1,RF)}  & 75.00\%                   & 68.00\%                   & 72.00\%                   & 70.00\%                    & 70.00\%                   & 59.00\%                   & 63.00\%                    \\
\multicolumn{1}{|c|}{S(B1,SB)}  & 72.00\%                   & 56.00\%                   & 28.00\%                   & 69.00\%                    & 85.00\%                   & 68.00\%                   & 32.00\%                    \\
\multicolumn{1}{|c|}{S(B1,ST)}  & 81.00\%                   & 31.00\%                   & 79.00\%                   & 83.00\%                    & 87.00\%                   & 41.00\%                   & 83.00\%                    \\
\multicolumn{1}{|c|}{S(B1,VF)}  & 57.00\%                   & 58.00\%                   & 60.00\%                   & 58.00\%                    & 72.00\%                   & 79.00\%                   & 77.00\%                    \\
\multicolumn{1}{|c|}{S(B5,BVT)} & 58.00\%                   & 50.00\%                   & 64.00\%                   & 33.00\%                    & 86.00\%                   & 70.00\%                   & 83.00\%                    \\
\multicolumn{1}{|c|}{S(B5,RF)}  & 62.00\%                   & 52.00\%                   & 56.00\%                   & 61.00\%                    & 73.00\%                   & 60.00\%                   & 67.00\%                    \\
\multicolumn{1}{|c|}{S(B5,SB)}  & 64.00\%                   & 45.00\%                   & 18.00\%                   & 57.00\%                    & 83.00\%                   & 70.00\%                   & 45.00\%                    \\
\multicolumn{1}{|c|}{S(B5,ST)}  & 73.00\%                   & 20.00\%                   & 63.00\%                   & 68.00\%                    & 87.00\%                   & 48.00\%                   & 78.00\%                    \\
\multicolumn{1}{|c|}{S(B5,VF)}  & 46.00\%                   & 50.00\%                   & 46.00\%                   & 40.00\%                    & 72.00\%                   & 69.00\%                   & 78.00\%                    \\
\multicolumn{1}{|c|}{S(RF,BVT)} & 77.00\%                   & 66.00\%                   & 71.00\%                   & 37.00\%                    & 70.00\%                   & 58.00\%                   & 61.00\%                    \\
\multicolumn{1}{|c|}{S(RF,SB)}  & 80.00\%                   & 69.00\%                   & 42.00\%                   & 77.00\%                    & 64.00\%                   & 50.00\%                   & 26.00\%                    \\
\multicolumn{1}{|c|}{S(RF,ST)}  & 90.00\%                   & 43.00\%                   & 79.00\%                   & 85.00\%                    & 80.00\%                   & 38.00\%                   & 71.00\%                    \\
\multicolumn{1}{|c|}{S(RF,VF)}  & 42.00\%                   & 58.00\%                   & 57.00\%                   & 39.00\%                    & 38.00\%                   & 49.00\%                   & 46.00\%                    \\
\multicolumn{1}{|c|}{S(SB,BVT)} & 82.00\%                   & 59.00\%                   & 49.00\%                   & 48.00\%                    & 84.00\%                   & 68.00\%                   & 35.00\%                    \\
\multicolumn{1}{|c|}{S(SB,ST)}  & 91.00\%                   & 42.00\%                   & 68.00\%                   & 89.00\%                    & 89.00\%                   & 41.00\%                   & 55.00\%                    \\
\multicolumn{1}{|c|}{S(ST,BVT)} & 92.00\%                   & 45.00\%                   & 86.00\%                   & 55.00\%                    & 90.00\%                   & 46.00\%                   & 81.00\%                    \\
\multicolumn{1}{|c|}{S(VF,BVT)} & 60.00\%                   & 62.00\%                   & 66.00\%                   & 32.00\%                    & 61.00\%                   & 74.00\%                   & 73.00\%                    \\
\multicolumn{1}{|c|}{S(VF,SB)}  & 79.00\%                   & 64.00\%                   & 37.00\%                   & 72.00\%                    & 79.00\%                   & 58.00\%                   & 43.00\%                    \\
\multicolumn{1}{|c|}{S(VF,ST)}  & 88.00\%                   & 38.00\%                   & 82.00\%                   & 78.00\%                    & 83.00\%                   & 35.00\%                   & 76.00\%                    \\ \hline
\end{tabular}
\end{table}

\begin{table}[]
\begin{tabular}{|crrrrrrr|}
\hline
\multicolumn{8}{|c|}{Full $\text{GaME}_2$ Table (CIFAR-10, $F_h$)}                                                                                                                                                                                                               \\ \hline
\multicolumn{1}{|c|}{Attack}    & \multicolumn{1}{l}{RF+BVT} & \multicolumn{1}{l}{VF+ST} & \multicolumn{1}{l}{VF+SB} & \multicolumn{1}{l}{VF+BVT} & \multicolumn{1}{l}{ST+SB} & \multicolumn{1}{l}{ST+BVT} & \multicolumn{1}{l|}{SB+BVT} \\
\multicolumn{1}{|c|}{APGD(RF)}  & 59.00\%                    & 68.00\%                   & 69.00\%                   & 74.00\%                    & 56.00\%                   & 58.00\%                    & 63.00\%                     \\
\multicolumn{1}{|c|}{APGD(SB)}  & 79.00\%                    & 75.00\%                   & 42.00\%                   & 80.00\%                    & 35.00\%                   & 65.00\%                    & 37.00\%                     \\
\multicolumn{1}{|c|}{APGD(ST)}  & 90.00\%                    & 47.00\%                   & 83.00\%                   & 91.00\%                    & 41.00\%                   & 40.00\%                    & 86.00\%                     \\
\multicolumn{1}{|c|}{APGD(VF)}  & 52.00\%                    & 39.00\%                   & 40.00\%                   & 25.00\%                    & 59.00\%                   & 38.00\%                    & 37.00\%                     \\
\multicolumn{1}{|c|}{MIME(B1)}  & 82.00\%                    & 77.00\%                   & 90.00\%                   & 93.00\%                    & 78.00\%                   & 79.00\%                    & 85.00\%                     \\
\multicolumn{1}{|c|}{MIME(B5)}  & 79.00\%                    & 77.00\%                   & 90.00\%                   & 89.00\%                    & 69.00\%                   & 71.00\%                    & 79.00\%                     \\
\multicolumn{1}{|c|}{MIME(BVT)} & 47.00\%                    & 79.00\%                   & 86.00\%                   & 54.00\%                    & 72.00\%                   & 41.00\%                    & 43.00\%                     \\
\multicolumn{1}{|c|}{S(B1,B5)}  & 86.00\%                    & 84.00\%                   & 90.00\%                   & 89.00\%                    & 76.00\%                   & 80.00\%                    & 86.00\%                     \\
\multicolumn{1}{|c|}{S(B1,BVT)} & 52.00\%                    & 80.00\%                   & 87.00\%                   & 59.00\%                    & 67.00\%                   & 47.00\%                    & 48.00\%                     \\
\multicolumn{1}{|c|}{S(B1,RF)}  & 64.00\%                    & 75.00\%                   & 83.00\%                   & 85.00\%                    & 68.00\%                   & 72.00\%                    & 79.00\%                     \\
\multicolumn{1}{|c|}{S(B1,SB)}  & 81.00\%                    & 72.00\%                   & 47.00\%                   & 90.00\%                    & 27.00\%                   & 63.00\%                    & 38.00\%                     \\
\multicolumn{1}{|c|}{S(B1,ST)}  & 83.00\%                    & 51.00\%                   & 88.00\%                   & 86.00\%                    & 45.00\%                   & 44.00\%                    & 81.00\%                     \\
\multicolumn{1}{|c|}{S(B1,VF)}  & 73.00\%                    & 62.00\%                   & 74.00\%                   & 74.00\%                    & 71.00\%                   & 68.00\%                    & 75.00\%                     \\
\multicolumn{1}{|c|}{S(B5,BVT)} & 57.00\%                    & 76.00\%                   & 91.00\%                   & 62.00\%                    & 68.00\%                   & 53.00\%                    & 53.00\%                     \\
\multicolumn{1}{|c|}{S(B5,RF)}  & 66.00\%                    & 76.00\%                   & 77.00\%                   & 81.00\%                    & 68.00\%                   & 67.00\%                    & 74.00\%                     \\
\multicolumn{1}{|c|}{S(B5,SB)}  & 75.00\%                    & 69.00\%                   & 51.00\%                   & 86.00\%                    & 34.00\%                   & 61.00\%                    & 36.00\%                     \\
\multicolumn{1}{|c|}{S(B5,ST)}  & 81.00\%                    & 53.00\%                   & 83.00\%                   & 91.00\%                    & 37.00\%                   & 47.00\%                    & 83.00\%                     \\
\multicolumn{1}{|c|}{S(B5,VF)}  & 62.00\%                    & 66.00\%                   & 70.00\%                   & 65.00\%                    & 68.00\%                   & 63.00\%                    & 66.00\%                     \\
\multicolumn{1}{|c|}{S(RF,BVT)} & 31.00\%                    & 72.00\%                   & 78.00\%                   & 46.00\%                    & 65.00\%                   & 39.00\%                    & 35.00\%                     \\
\multicolumn{1}{|c|}{S(RF,SB)}  & 58.00\%                    & 60.00\%                   & 38.00\%                   & 76.00\%                    & 29.00\%                   & 61.00\%                    & 24.00\%                     \\
\multicolumn{1}{|c|}{S(RF,ST)}  & 78.00\%                    & 45.00\%                   & 80.00\%                   & 91.00\%                    & 41.00\%                   & 44.00\%                    & 78.00\%                     \\
\multicolumn{1}{|c|}{S(RF,VF)}  & 39.00\%                    & 45.00\%                   & 41.00\%                   & 31.00\%                    & 51.00\%                   & 46.00\%                    & 40.00\%                     \\
\multicolumn{1}{|c|}{S(SB,BVT)} & 49.00\%                    & 75.00\%                   & 38.00\%                   & 48.00\%                    & 31.00\%                   & 37.00\%                    & 11.00\%                     \\
\multicolumn{1}{|c|}{S(SB,ST)}  & 87.00\%                    & 50.00\%                   & 63.00\%                   & 92.00\%                    & 18.00\%                   & 48.00\%                    & 66.00\%                     \\
\multicolumn{1}{|c|}{S(ST,BVT)} & 56.00\%                    & 37.00\%                   & 87.00\%                   & 57.00\%                    & 43.00\%                   & 10.00\%                    & 39.00\%                     \\
\multicolumn{1}{|c|}{S(VF,BVT)} & 35.00\%                    & 57.00\%                   & 63.00\%                   & 16.00\%                    & 65.00\%                   & 34.00\%                    & 31.00\%                     \\
\multicolumn{1}{|c|}{S(VF,SB)}  & 67.00\%                    & 59.00\%                   & 41.00\%                   & 69.00\%                    & 24.00\%                   & 53.00\%                    & 28.00\%                     \\
\multicolumn{1}{|c|}{S(VF,ST)}  & 83.00\%                    & 39.00\%                   & 80.00\%                   & 76.00\%                    & 40.00\%                   & 33.00\%                    & 78.00\%                     \\ \hline
\end{tabular}
\end{table}
